# Supplementary material for: Riemann-Silberstein geometric phase in 4D polarization space
Source: arXiv:2510.09112 source file (2025-11-17)
Supplement: Supplementary file 1 [file SI.tex]

\documentclass{article}
\usepackage{pdfpages}

\begin{document}
\includepdf[pages=-]{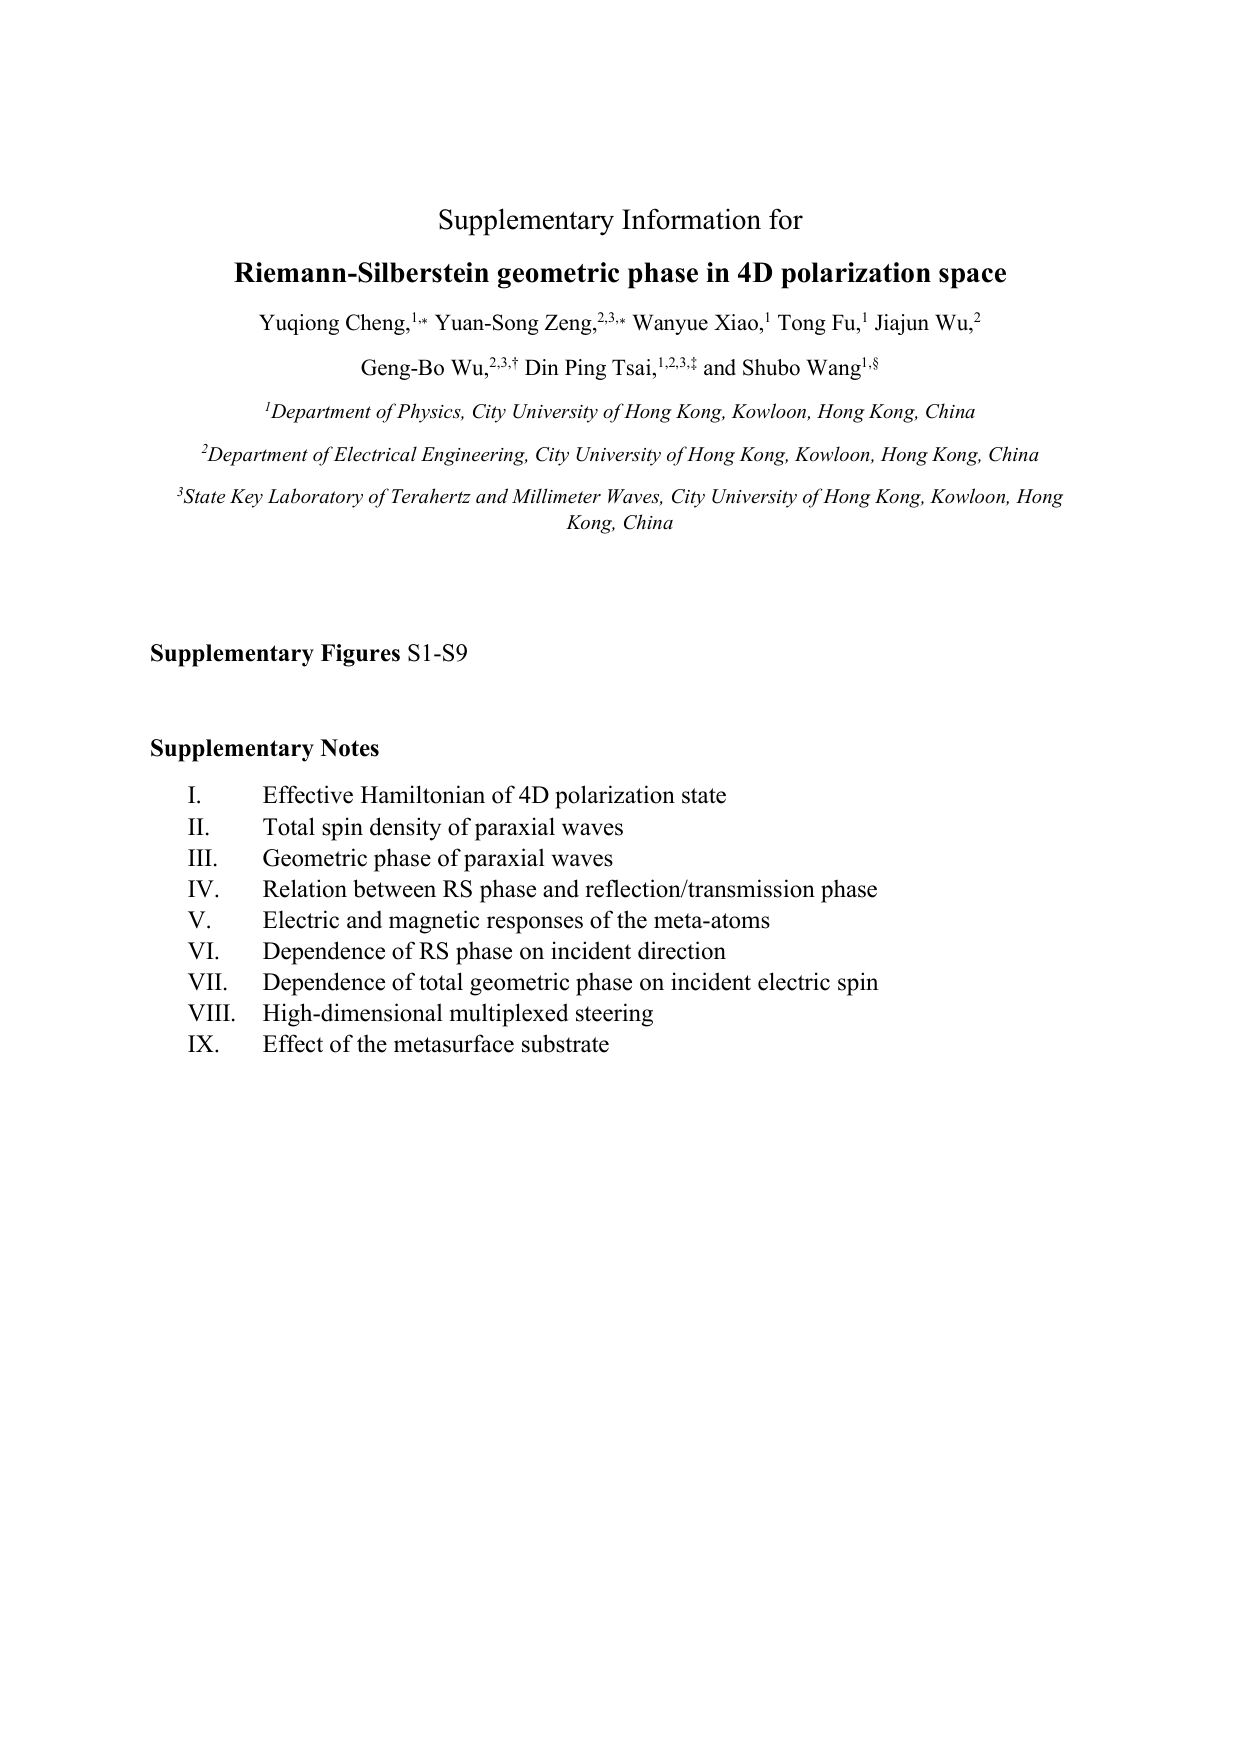}
\end{document}
